# Supplementary material for: Emergence of molecular friction in liquids: bridging between the atomistic and hydrodynamic pictures
Source: arXiv:2004.07631 ancillary file (2020-04-16)
Supplement: Supplementary file 1 [file dynamic-friction-suppl.pdf]

# Supplemental material on “Emergence of molecular friction in liquids: bridging between the atomistic and hydrodynamic pictures”

Arthur V. Straube,[1,2] Bartosz G. Kowalik,[3] Roland R. Netz,[3] and Felix Höfling[1,2]
[1)] *Freie Universität Berlin, Department of Mathematics and Computer Science, Arnimallee 6, 14195 Berlin, Germany*
[2)] *Zuse Institute Berlin, Takustr. 7, 14195 Berlin, Germany*
[3)] *Freie Universität Berlin, Department of Physics, Arnimallee 14, 14195 Berlin, Germany*

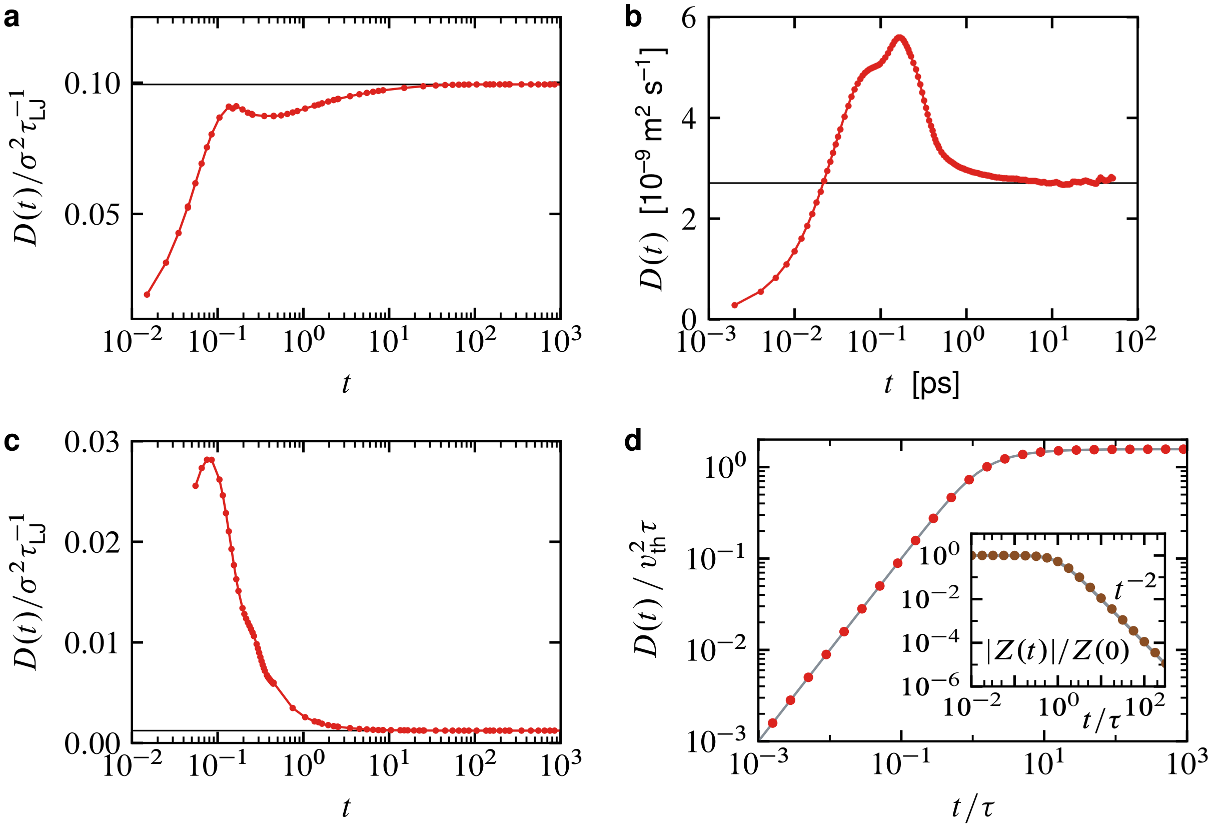


FIG. S1. Timescale-dependent diffusion coefficient $D(t) = \partial_t \mathrm{MSD}(t)/6$ for (panel a) a Lennard-Jones fluid, (b) liquid water, (c) a supercooled Kob–Andersen mixture, and (d) the analytically solvable example. In panel (d), symbols represent data points used for the numerics (only every 5th point is drawn for clarity), solid lines correspond to the analytical expressions.

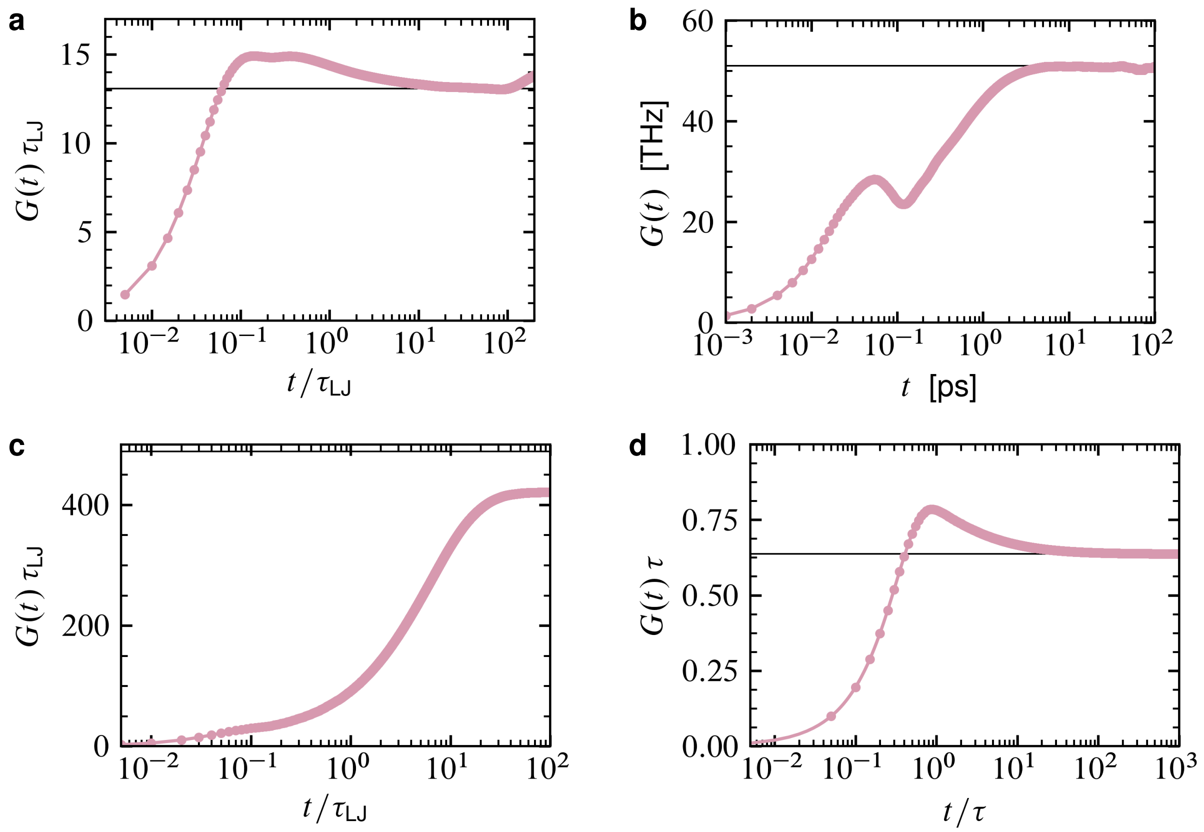


FIG. S2. Integral $G(t) = \int_0^t \gamma(s)\,\mathrm{d}s$ of the memory function for (panel a) a Lennard-Jones fluid, (b) liquid water, (c) a supercooled Kob–Andersen mixture, and (d) the analytically solvable example. The long-time limit $G(t \to \infty) = \zeta_0/m$ is indicated by the horizontal line.
